# Supplementary material for: A Leap among Quantum Computing and Quantum Neural Networks: A Survey
Source: arXiv:2107.03313 source file (2022-01-31)
Supplement: Supplementary file 1 [file x_entanglement.tex]

\subsection{Entanglement} \label{app:entanglement}

The Entanglement~\citep{guhne2009entanglement,lanting2014entanglement,smirnov2013ground} is among the most relevant quantum mechanical phenomenon for quantum computing and information theories. Indeed, as reported in~\citep{preskill2012quantum}: ``At the core of quantum information science is entanglement, the characteristic correlations among the parts of a quantum system, which have no classical analog". 

The Entanglement does not have a classical analogous and due to its extravagant, and at the same fascinating, properties it has been the core of several scientific debates, especially since at the beginning it seemed it was in contrast with the theory of special relativity~\citep{einstein1935can,aspect1999bell}. By using a non-formal language, one can consider an entangled system as made of several, different, subsystems that acts as they were a single entity, i.e., an interaction on a single subsystem affects the state of the whole system. It is a correlation between the various subsystems that manifests itself by making the probability for obtaining a certain value for the observable of one subsystem depending on the state of the other subsystems. 

Although it plays a key role in all the quantum computation and information theories, and since we notice that such a topic is skipped in almost the surveys on quantum computation, we decide to offer to the reader a brief introduction on such a phenomenon giving a grasp of the basics theoretical notions beneath the entanglement.
