# Supplementary material for: A Leap among Quantum Computing and Quantum Neural Networks: A Survey
Source: arXiv:2107.03313 source file (2022-01-31)
Supplement: Supplementary file 6 [file x_entanglement_old.tex]

\subsection{Entanglement} \label{app:entanglement}

The Entanglement~\citep{guhne2009entanglement,lanting2014entanglement,smirnov2013ground} is among the most relevant quantum mechanical phenomenon for quantum computing and information theories. Indeed, as reported in~\citep{preskill2012quantum}: ``At the core of quantum information science is entanglement, the characteristic correlations among the parts of a quantum system, which have no classical analog". 

The Entanglement does not have a classical analogous and due to its extravagant, and at the same fascinating, properties it has been the core of several scientific debates, especially since at the beginning it seemed it was in contrast with the theory of special relativity~\citep{einstein1935can,aspect1999bell}. By using a non-formal language, one can consider an entangled system as made of several, different, subsystems that acts as they were a single entity, i.e., an interaction on a single subsystem affects the state of the whole system. It is a correlation between the various subsystems that manifests itself by making the probability for obtaining a certain value for the observable of one subsystem depending on the state of the other subsystems. 

Although it plays a key role in all the quantum computation and information theories, and since we notice that such a topic is skipped in almost the surveys on quantum computation, we decide to offer to the reader a brief introduction on such a phenomenon giving a grasp of the basics theoretical notions beneath the entanglement.

To begin with, we consider two systems, namely $\Phi$ and $\Psi$, and assume that a generic state of the overall systems, namely $\Theta$, can be expressed as the tensor product $|\phi_i\rangle|\psi_j\rangle$, where $|\phi_i\rangle$ and $|\psi_j\rangle$ are basis states for two systems. Moreover, we refer to $\Theta$ as the ``composite'' system, and we indicate a generic state for the composite system as $|\Theta; i,j \rangle$, indicating that the subsystem $\Phi$ and $\Psi$ are in the $i$-th and $j$-th state, i.e., $\ket{\phi_i}$ and $\ket{\psi_j}$, respectively. By defining the corresponding bras as %$\langle\phi_i|\langle\psi_j|$
$\bra{\phi_i}$ and $\bra{\psi_j}$, we can evaluate the probability of finding $\Theta$ in the state $|\Theta; k,l \rangle$ as:

\begin{equation} \label{eq:ent1}
p(|\Theta; k,l \rangle) = | \langle\Theta; k,l |\Theta; i,j \rangle |^2 = 
|\langle \phi_k | \phi_i \rangle|^2|\langle \psi_l | \psi_j \rangle|^2 = p(|\phi_k \rangle)p(|\psi_l \rangle)
\end{equation}
% \begin{equation} \label{eq:ent1}
% p(|\Theta; k,l \rangle) = \sum_{i,j}| \langle\Theta; k,l |\Theta; i,j \rangle |^2 = \sum_{i,j}
% |\langle \phi_k | \phi_i \rangle|^2|\langle \psi_l | \psi_j \rangle|^2 = p(|\phi_k \rangle)p(|\psi_l \rangle)
% \end{equation}
where $p(|\phi_k \rangle)$ and $p(|\psi_l \rangle)$ are the probability of finding the systems $\Phi$ and $\Psi$ in the states $k$-th and $l$-th, respectively. Thus, we have been able to express a generic state of $\Theta$ as the product of states of the two subsystems. Before to draw our first conclusions, let us consider a concrete example. Assume that $\{|\psi_i\rangle\} = \{|\uparrow\rangle; |\downarrow\rangle\}$ and $\{|\phi_i\rangle\} = \{|+\rangle; |-\rangle\}$. Thus, we can define the generic state for the two subsystems and for the composite one as:

\begin{align*}\label{eq:ent2}
|\Psi\rangle &= a_{\uparrow} |\uparrow\rangle + a_{\downarrow} |\downarrow\rangle \ \ \ ; \ \ \ 
|\Phi\rangle = b_{+} |+\rangle + b_{-} |-\rangle \\ 
|\Theta\rangle &= |\Psi\rangle|\Phi\rangle = a_{\uparrow}b_{+} |\uparrow\rangle|+\rangle + a_{\downarrow}b_{+} |\downarrow\rangle|+\rangle + a_{\uparrow}b_{-} |\uparrow\rangle|-\rangle + a_{\downarrow}b_{-} |\downarrow\rangle|-\rangle \numberthis 
\end{align*}

where the coefficients $a_i$ and $b_j$ represent the amplitudes for the subsystems to be in the $i$-th and $j$-th state, respectively. With such a representations, the probability of finding the $\Phi$ in the $|+\rangle$ with $\Psi$ in either the up- or downstate, is given by $p_{+\uparrow}/p_{+\downarrow} = |b_\uparrow|^2/|b_\downarrow|^2$. Subsequently, the probability of finding $\Psi$ in the $|\uparrow\rangle$ given that $\Phi$ is in its $|+\rangle$ state is given by: 

\begin{equation} \label{eq:ent3}
p(|\uparrow\rangle | | +\rangle) = \frac{p_{+ \uparrow}}{p_{+}} = \frac{p_{+ \uparrow}}{p_{+ \uparrow}+p_{+ \downarrow}} = \frac{1}{1+p_{+\downarrow}/p_{+\uparrow}} = \frac{1}{1 + |b_\downarrow/b_\uparrow|^2}
\end{equation}

Thus, when we can express the composite system as a mere product of the states of the subsystems, the probability of finding one in a state, e.g., $|\uparrow\rangle$, is independent from the states of the other systems. From~\autoref{eq:ent1} and~\autoref{eq:ent3}, we conclude that when the state of a system can be described by a product of the subsystems' state, then the subsytems are said uncorrelated or statistically independent. Specifically, we notice that to describe the state of the composite system, we only need $N+M$ coefficients, where $N$ and $M$ represent the dimension of the Hilbert spaces for the systems $\Phi$ and $\Psi$, respectively.

The more general form to describe a generic state $\theta$ of the composite system is given by:

\begin{equation} \label{eq:ent4}
|\theta \rangle = \sum_{ij} c_{ij} |\Theta; ij\rangle = \sum_{ij} c_{ij} | \Psi; i\rangle |\Phi; j\rangle  
\end{equation}

where $c_{ij}$ are entries of a $N \times M$ matrix. Thus,~\autoref{eq:ent2} represents a specific instance of the given problem, i.e., it is the case when we can express the states of the composite system as a product of states of the subsystems. That simply means that, the coefficients $c_{ij}$ are given by the external product between a vector of size $N$ and one of size $M$. Specifically, if we consider such a case, we obtain that $c_{ij}/c_{ik} = a_ib_j/a_ib_k=b_j/b_k$. Thus, the $N \times M$ matrix of the $c_{ij}$ coefficients, is such that each row is a multiple of the first one. Analogous reasons hold for the columns. Whenever those conditions are not met, then the subsytems are said to be entangled. For example, there is no way to express the state:

\begin{equation} \label{eq:ent5}
|\theta \rangle = \alpha_1|+\rangle|\uparrow\rangle + \alpha_2|-\rangle|\uparrow\rangle + \alpha_3 |-\rangle|\uparrow\rangle  
\end{equation}

 as the product $|\Psi\rangle|\Phi\rangle$.

Let us now see how it is possible to develop entanglement among states. As we saw previously that, in the case non-entangled systems, the probability for the system $\Psi$ for being in the $|\uparrow\rangle$ state is not affected by the status of system $\Phi$, thus they are statistical independent. Especially, such a picture characterizes systems that are non-interacting, i.e., the Hamiltonian of the whole system is simply given as the sum of the Hamiltonian for the single subsytems which automatically translates into saying that there is a common set of eigenvectors for the single as well as to the total Hamiltonian operators. For example, assume the following structure for the Hamiltonians:

\begin{align*} 
H_{\Theta} = H_{\Psi} + H_{\Phi} = \frac{p^2_{|\Psi\rangle}}{2 m_{|\Psi\rangle}} + \frac{p^2_{|\Phi\rangle}}{2 m_{|\Phi\rangle}} \numberthis \label{eq:ent_hamilt}
\end{align*}

then, it is easily checked that 

\begin{align*} 
\langle \phi_i \psi_j | (H_{\Psi} + H_{\Phi}) | \phi_m \psi_n \rangle &= \langle \phi_i | H_{\Phi} | \phi_m \rangle \langle \psi_j | \psi_n \rangle + \langle \psi_j | H_{\Psi} | \psi_n \rangle \langle \phi_i | \phi_m \rangle \\ \numberthis \label{eq:ent_avg_hamilt}
&= \langle \phi_i | H_{\Phi} | \phi_m \rangle \delta_{jn} + \langle \psi_j | H_{\Psi} | \psi_n \rangle \delta_{im}
\end{align*}

thus, by setting $j=n$ and $i=m$ one obtains the energy of the whole system as the sum of the kinetic energies of the its components. Most important, from~\autoref{eq:ent_avg_hamilt} we see that the Hamiltonian of system $\Psi$ does not have any effect on the system $\Phi$ whatsoever, and vice versa. With such a premise, we can write the Time-Dependent Schr{\"o}dinger Equation (TDSE) as:

\begin{align*}
i \hbar \frac{\partial |\Phi\Psi\rangle}{\partial t} &= i \hbar \frac{\partial}{\partial t} |\Phi\rangle|\Psi\rangle = i \hbar \bigg( \frac{\partial |\Phi\rangle}{\partial t}|\Psi\rangle + |\Phi\rangle \frac{\partial|\Psi\rangle}{\partial t} \bigg) \\
&= (H_{\Phi}|\Phi\rangle)|\Psi\rangle + |\Phi\rangle(H_{\Psi}|\Psi\rangle) \\
&= (H_{\Phi} + H_{\Psi})|\Phi\rangle|\Psi\rangle \\
&= H_{\Theta}|\Phi\rangle|\Psi\rangle \numberthis \label{eq:ent_tdse}
\end{align*}

In such a situation we are describing two non-intercating, and non-entangled, systems. Let us now turn an interactions among them. The Hamiltonian of the composite system is no longer given by the sum of the single Hamiltonians. Specifically, $H_{\Theta} = H_{\Phi} + H_{\Psi} \rightarrow H_{\Phi} + H_{\Psi} + H_{\mathrm{int}}$. If one apllies the new Hamiltonians to~\autoref{eq:ent4}, it obtains:

\begin{equation}\label{eq:ent6}
i\hbar \sum_{ij}\frac{dc_{ij}}{dt}|\psi_i\rangle|\phi_j\rangle = \sum_{ij}c_{ij}H_{\mathrm{int}}|\psi_i\rangle|\phi_j\rangle
\end{equation}

where we can see that the evolution of the coefficients is directly related to the interaction Hamiltonian, i.e., if $H_{\mathrm{int}}=0$, then there is no interactons, so if the system is initially unentangled it remains so. To see this, let us bra through the~\autoref{eq:ent6}: 

\begin{equation}\label{eq:ent7}
i\hbar \frac{dc_{kl}}{dt} = \sum_{ij}c_{ij} \langle \phi_k \psi_l | H_{\mathrm{int}} | \phi_i \psi_j \rangle = \sum_{ij}c_{ij} H_{\mathrm{int}}^{kl;ij}
\end{equation}

In~\autoref{eq:ent7}, the term $H_{\mathrm{int}}^{kl;ij}$ describes the matrix that encapsulates the time variation of the $c_{kl}$ coefficient. Let us assume that all the elements are 0 except for the element $\langle \phi_{k_{0}} \psi_{l_{0}} | H_{\mathrm{int}} | \phi_{i_{0}} \psi_{j_{0}} \rangle$ that sits on the diagonal, meaning that only the coefficient $c_{k_0l_0}$ has a non-vanishing time derivative. As we saw at the beginning of this subsection, the condition for two systems for being non-entangled was that the ratio $c_{ij}/c_{ik}$ was independent from $i$. Concerning the current case, when $t=0$ such a condition is satisfied. However, as soon as the interaction among the systems is turned on, the ratio $c_{k_0l_0}/c_{k_0m}$ violates such a condition for $m \neq l_0$. Thus, after a certain amount of time the state of one subsystem has become dependent on the state of the other, i.e., the two states are now correlated or entangled.
